# Supplementary material for: OpenCarbon: A Contrastive Learning-based Cross-Modality Neural Approach for High-Resolution Carbon Emission Prediction Using Open Data
Source: arXiv:2506.03224 source file (2025-06-03)
Supplement: Supplementary file 1 [file experiment.tex]

\subsection{Experimental Setups}
\subsubsection{Dataset}
We select three representative regions from both developing and developed countries for comprehensive evaluation: Beijing, Great London, and New York. For Beijing, we selected the six most central districts as our dataset. Table~\ref{tbl:dataset} summarizes the basic information of the three datasets. For each city, we collect its carbon emission statistics from ODIAC~\cite{oda2018open}, a well-acknowledged carbon emission inventory constructed using the hybrid means of point emission calculations and top-down allocations. Consistent with ODIAC, we set our prediction resolution as 1km $\times$ 1km, which is the highest resolution in the existing works. In our training, we randomly split the dataset into 60\% training dataset, 20\% validation dataset, and 20\% test dataset.

\begin{table}[h]
    \caption{The summary statistics of our datasets.}~\label{tbl:dataset}
    \centering
    \scalebox{0.95}{
    \begin{tabular}{l c c c}
        \toprule
        Region & Beijing & Great London & New York City \\
        \midrule
        Area & $1381 km^2$ & $778 km^2$ & $1569 km^2$ \\
        POI Source & Tencent Map & SafeGraph & SafeGraph \\
        Target Year & 2018 & 2018 & 2019 \\
        \#POI Categories& 14 & 14 & 15 \\
        \bottomrule
    \end{tabular}}
\end{table}

\subsubsection{Baselines}
Since our task is to predict carbon emissions with open data, we compare our models with both existing carbon emission prediction methods and methods that predict socioeconomic indicators with open data. Existing carbon emission prediction methods typically incorporate machine learning or neural network methods to capture the correlations between attributes and carbon emissions, such as:
\begin{itemize}[leftmargin=*]
    \item \textbf{SVM}~\cite{mladenovic2016management}. Support vector machine method that effectively identifies a hyperplane with the maximum margin to separate data points in different classes.
    \item \textbf{Stacked-RFR}~\cite{zhang2022estimating}. An ensemble machine learning technique that introduces a two-layer stacked random forest regression model to improve predictive performance.
    \revision{\item \textbf{BPNN}~\cite{zhang2021towards}. A classical back propagation neural network that fits prediction targets with given attributes.}
    \item \revision{\textbf{CarbonGCN}~\cite{chen2024spatiotemporal}. A graph neural network with graph convolutional layers to predict carbon emissions considering correlations between connected grids.}
\end{itemize}
For these carbon prediction methods, we input the satellite image representation whose dimension is reduced by PCA~\cite{tipping1999probabilistic} and the facility distribution vector as attributes in our implementation.

We further compare with several state-of-the-art baselines that involve utilizing open data to make socioeconomic predictions, mainly using satellite images:
\begin{itemize}[leftmargin=*]
    \item \textbf{ResNet-18}~\cite{yeh2020using, he2016deep}. A classical convolutional neural network design for practical image-related tasks.
    \item \textbf{READ}~\cite{han2020lightweight}. A pretrained satellite image representation model trained with transfer learning methods on a large-scale partially-labeled dataset to learn robust and lightweight satellite image representations. We directly use the embedding model of the original paper to represent satellite images and train a random forest model for final prediction.  
    \item \textbf{Tile2Vec}~\cite{jean2019tile2vec}. Following the first law of geography that near things are more similar than distant ones, Tile2Vec uses triplet loss to maximize the representation similarity of satellite images of geo-adjacent pairs and minimize that of geo-distant pairs.   
    \item \textbf{PG-SimCLR}~\cite{xi2022beyond}. A satellite image representation method where grids with similar facility distribution and geo-adjacent grids are encouraged to have similar representation by the self-supervised SimCLR~\cite{chen2020simple} model. 
\end{itemize}
Since our task is a supervised learning task, for a fair comparison, we transform the unsupervised Tile2Vec and self-supervised PG-SimCLR into a supervised solution. Specifically, we add the loss term of predicting carbon emission with the representations to the original representation learning losses of these models and balance the multiple loss terms. For all these socioeconomic prediction studies, we also input the facility distribution information at the prediction stage by concatenating the learned image representation and the POI count vector as prediction input.

\subsubsection{Metrics and Implementation}
To measure the prediction performance, we adopt three commonly used evaluation metrics: mean absolute error (MAE), rooted mean squared error (RMSE), and coefficient of determination ($R^2$)~\cite{xi2022beyond, jean2016combining}. 

Since the absolute value of carbon emission is large, we take its logarithmic value as our prediction target. For the implementation, we apply Adam optimizer for parameter learning. We perform a grid search on all hyperparameters, including learning rate and batch size for our model and all baselines. The grid search range for learning rate is set as \{5e-6, 1e-5, 5e-5, 1e-4, 5e-4, 1e-3, 5e-3, 1e-2\}, and the range for batch size is \{32, 64, 128\}. We also finetune the size of the neighborhood $M$ in the range of \{3, 5, 7\}. We set the number of epochs as 500, with an early stopping mechanism to prevent overfitting. Meanwhile, we also fine-tune all hyperparameters of the baselines for fair comparisons. 
% The implementation codes are available at this link~\footnote{https://github.com/JinweiZeng/OpenCarbon}.

\subsection{Transferability Study}

\revision{Unlike other common socioeconomic indicators, transferability of carbon emission prediction model faces the extremely severe challenge of distribution shift since multiple factors besides human behavior, including temperature, precipitation, and energy structure, will all impact a region’s carbon emission level. Therefore, to comprehensively figure out how to transfer our model in different situations, we research into the transferability under two scenarios: transfer between regions with similar attribute conditions, and transfer between regions with significant attribute differences. The key attributes of all regions involved are summarized in Table~\ref{tbl:transfer dataset}.}

\begin{table*}[h]
    \caption{Basic statistics of the transferred regions}~\label{tbl:transfer dataset}
    \centering
    \scalebox{0.95}{
    \begin{tabular}{l c c c c}
        \toprule
        Region & Great London & Great Manchester & West Midlands & South Yorkshire \\
        \midrule
        Average Temperature (°C) & 10.8 & 9.4& 9.7 & 9.2 \\
        Average Precipitation (mm) & 690 & 1047 & 769& 864\\
        Population Density (/km^2) &5,671 & 2,204 & 3,235 & 912\\
        Per Capita GDP (\$) & 75,336 & 38,360 & 33,547 & 28,550 \\
        Average Grid Emissions (t) & 148.99 & 115.27& 110.24 & 45.84 \\
        \bottomrule
    \end{tabular}}
\end{table*}

\revision{\subsubsection{Transfer between regions with similar attributes}
We assess the transferability of our model using three comparable ceremonial counties in England: the Greater London region, the Greater Manchester region, and the West Midlands region. These areas are relatively more developed and have higher population densities, as indicated in Table~\ref{tbl:transfer dataset}. Consequently, all three regions exhibit similarly high levels of carbon emissions. We conduct transferability tests on the total six source-target pairs on both our model and the best baseline, PG-SimCLR. The results are shown in Figure~\ref{fig:transfer}.}

\begin{figure}[h]
    \vspace{-3mm}
    \centering
    \includegraphics[width=0.7\columnwidth]{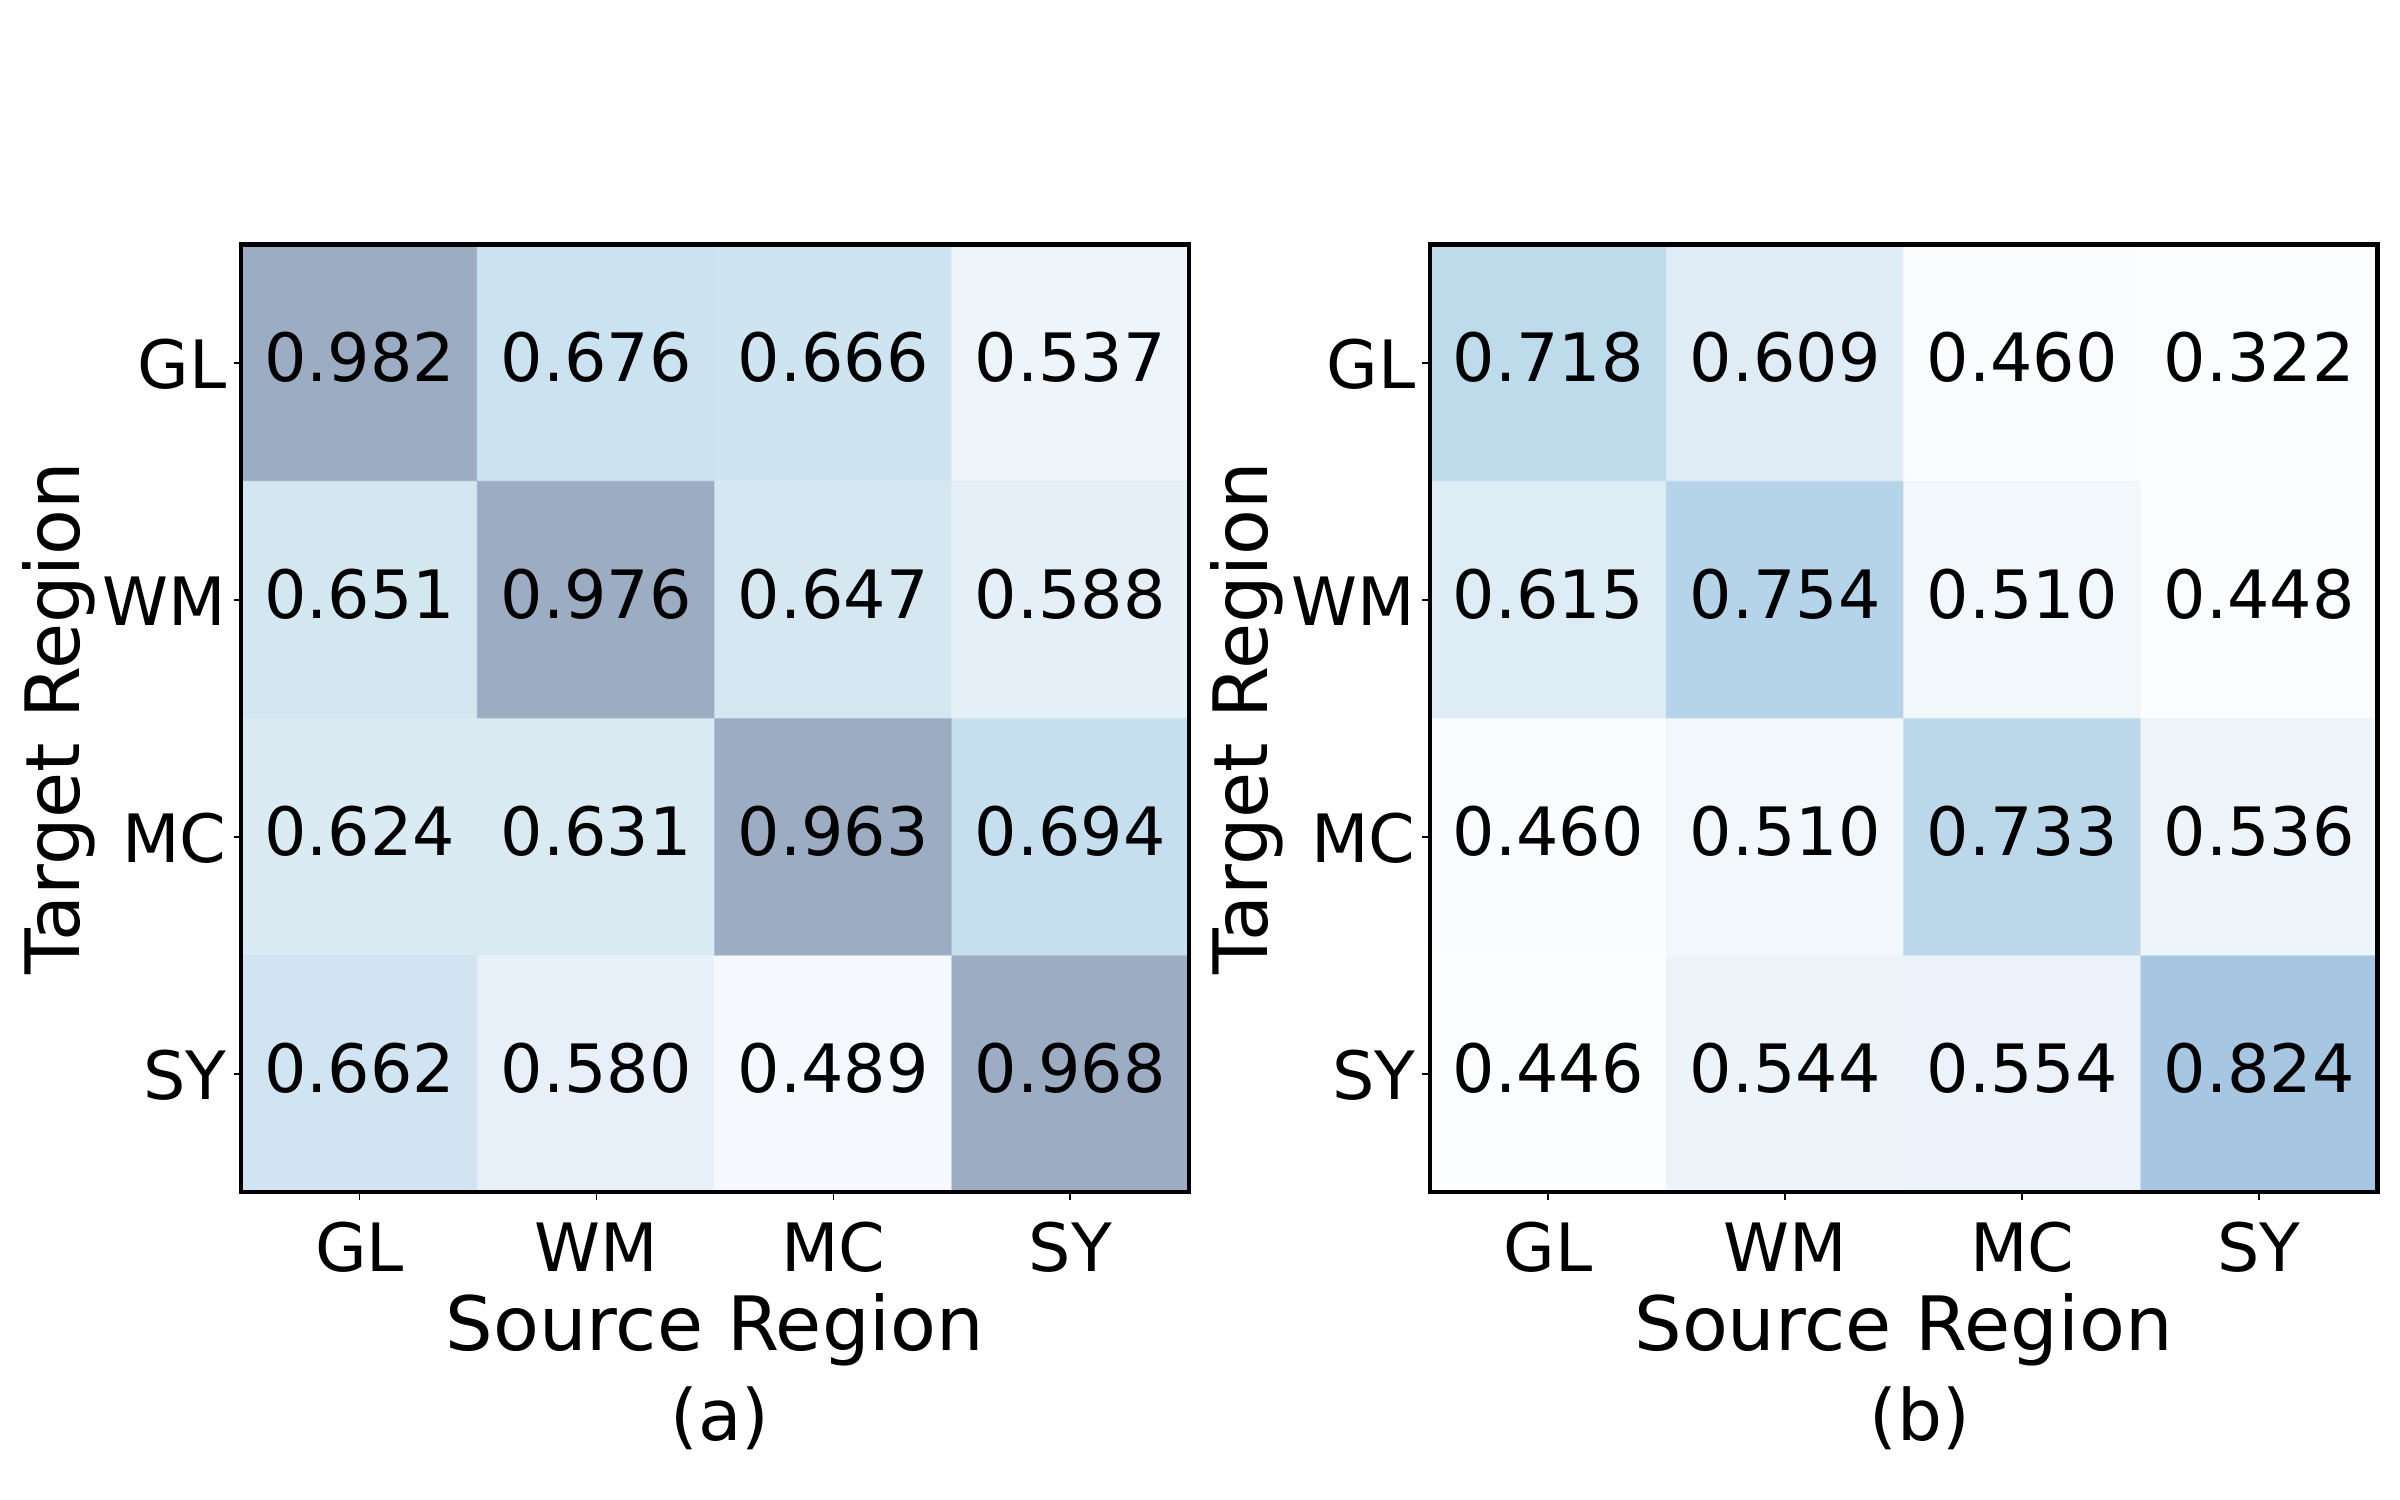}
    \caption{The $R^2$ for the transferability test on (a) our model and (b) PG-SimCLR on three England regions: Great London (GL), Great Manchester (GM), and West Midlands (WM).}
    \label{fig:transfer}
    % \vspace{-4mm}
\end{figure}

\revision{As depicted by Figure~\ref{fig:transfer}(a), our model achieves good performance for all the six source-target pairs, achieving an average $R^2$ accuracy of 0.5275. Also, the transferability performance is stable across different source-target pairs, which is an important strength in real applications. In contrast, the transferability performance of PG-SimCLR~\cite{xi2022beyond} is much worse. Our model outperforms PG-SimCLR by 93.3\% on $R^2$ on average. The performances of the PG-SimCLR also have great fluctuations.}

% The reasons behind the good transferability of our model may come from several aspects. On one hand, our model manages to extract the inclusive functional semantics with the cross-modality attentive module and models the relationship between carbon emission and functionality information. Therefore, although different regions have some differences in functionality compositions, the learned relationship between carbon emission and functionality information is transferable across regions. On the other hand, since the agglomeration effect of carbon emission is universal, our model's ability to capture the spatial interaction between grids helps the model quickly learn the general functionality distribution of the new region, thus having a good prediction performance on this new region.

\revision{\subsubsection{Transfer between regions with significant attribute differences}
However, for practical applicability, it is essential to evaluate the transferability between regions with significant attribute differences, especially considering the typical unavailability of data in less-developed regions and the necessity to transfer knowledge from developed regions to less-developed ones. Therefore, we conduct transferability tests between the three developed regions, Great London, Great Manchester, and West Midlands, and the relatively less-developed region, South Yorkshire, which has a sparser population and lower per capita GDP. The experimental results are listed in Table~\ref{tbl:transfer}.  }

\begin{table*}[h]
    \caption{Transferability between regions with significant attribute differences on $R^2$. Here $GL$ is short for Great London, $GM$ is short for Great Manchester, $WM$ is short for West Midlands, and $SY$ is short for South Yorkshire. (C) indicates the experimental results with calibration. }~\label{tbl:transfer}
    \centering
\scalebox{0.9}{
    \begin{tabular}{l c c c c c c}
        \toprule &$GL\rightarrow SY $&$GM\rightarrow SY$&$WM\rightarrow SY$&$SY\rightarrow GL$&$SY\rightarrow GM$&$SY\rightarrow WM$ \\
        \midrule
        PG-SimCLR & $-0.7431$ & $-0.2503$ &$-0.1963$ & $-0.5199$ & $-0.1480$  & $-0.5080$ \\
        Our Model &$-2.4801$&$-0.2112$&$-0.6484$ &$-0.6447$ & $-0.4143$  & $-0.4453$ \\
        \midrule
        PG-SimCLR (C)
        & $-0.1055$ & $0.2657$ &$0.1455$ & $0.1000$ & $0.3674$  & $-0.0238$ \\
        Our Model (C) & \bm{$0.3661$} & \bm{$0.6669$} &\bm{$0.4549$} & \bm{$0.6764$} & \bm{$0.6127$}  & \bm{$0.6655$} \\
        \bottomrule
    \end{tabular}
}
\end{table*}

\revision{As shown in Table~\ref{tbl:transfer}, directly transferring between regions with significant attribute differences leads to poor performance for both our method and PG-SimCLR~\cite{xi2022beyond}. This could be attributed to substantial variations in the distribution of carbon emission levels across these regions. However, the transferability results will lift substantially with the simple mean-deviation calibration shown in Equation~\ref{equ:calibration}. Here $\mu$ and $\sigma$ are the mean and standard deviation of the original prediction outputs $y$, and ${\mu}^{'}$ and ${\sigma}^{'}$ are those of the prediction targets.}

\begin{equation}
    \revision{\hat{y}=\frac{y-\mu}{\sigma}*{\sigma}^{'} + {\mu}^{'}}
    \label{equ:calibration}
\end{equation}

\revision{By leveraging the mean and standard deviation of carbon emissions in the target region to scale our transferability results, we can significantly enhance the performance of our model. Specifically, we achieve an average $R^2$ value of 0.5738, surpassing the calibrated PG-SimCLR model by an average margin of $0.4489$. Therefore, we can conclude that our model is more capable of predicting the relative carbon emission levels between grids, indicating that our model captures the inherent relationship between changes in land uses and POI distribution and carbon emission variations. Furthermore, given that city officials in practical scenarios must discern the relative carbon emission levels among various areas and subsequently target major polluters, our model effectively addresses this requirement. Thus, we can assert that our model demonstrates practical transferability across diverse regions, ranging from regions with similar attributes and distinct attributes.}

\subsection{Robustness of Prediction Resolution}
\begin{table*}[t]
    \caption{Experimental results on different prediction resolutions.}~\label{tbl:resolution}
    \centering
\scalebox{0.9}{
    \begin{tabular}{l c c c c c c c c c c c c}
        \toprule &\multicolumn{3}{c}{1km $\times$ 1km (2067 samples)} &&  
        \multicolumn{3}{c}{2km $\times$ 2km (541 samples)} &&  \multicolumn{3}{c}{3km $\times$ 3km (193 samples)} \\
        \cmidrule{2-4} \cmidrule{6-8} \cmidrule{10-12}
        Models & MAE & RMSE & $R^2$ && MAE & RMSE & $R^2$ && MAE & RMSE & $R^2$ \\
        \midrule
        PG-SimCLR & $0.3250$ & $0.4429$ &$0.7587$ && $0.4603$ & $0.6442$  & $0.5650$ 
        &&$0.5199$ & $0.7804$ &$0.5108$ \\
        Our Model &$0.1830$&$0.2348$&$0.9322$ &&$0.3333$ &$0.5213$&$0.7151$ &&$0.4600$&$	0.7646$&$0.5304$\\
        Improv. & $43.69\%$ & $46.99\%$ & $27.59\%$&& $19.08\%$ & $26.57\%$  &$32.89\%$ && $11.52\%$ & $2.02\%$ &$3.84\%$\\
        \bottomrule
    \end{tabular}
}
\end{table*}
In the main experiment, we predict the carbon emission with the resolution of 1km $\times$ 1km, which is the highest spatial resolution in existing carbon emission databases. In this part, we test the model robustness with different spatial resolutions, which can correspond to multiple levels of administrative divisions like street, community, county, city, etc. Specifically, we conduct experiments in Beijing, changing the spatial resolution across 1km $\times$ 1km to 2km $\times$ 2km and 3km $\times$ 3km, and the results are shown in Table~\ref{tbl:resolution}. In our experiments, the resolution of satellite images and facility distribution is aligned with the corresponding studied resolution.

According to the results in the table, our model outperforms the best baseline significantly across all resolutions, showing a performance gain of 27.59\%, 32.89\%, and 3.84\% for 1km $\times$ 1km to 2km $\times$ 2km and 3km $\times$ 3km resolution respectively. The decreasing number of samples, as the resolution decreases, may account for the slight decrease of performance gain on 3km $\times$ 3km resolution since there are not enough samples with large neighborhoods where we can learn spatial interactions between samples. Since our model's design that models the function effect and agglomeration effect works for targets of all resolutions, our model has robustness over multiple prediction resolutions, showing a promising potential to apply to different levels of administrative divisions.
