# Supplementary material for: OpenCarbon: A Contrastive Learning-based Cross-Modality Neural Approach for High-Resolution Carbon Emission Prediction Using Open Data
Source: arXiv:2506.03224 source file (2025-06-03)
Supplement: Supplementary file 2 [file experiment_new.tex]

\begin{table*}[ht]
    \caption{Basic statistics of the transferred regions}~\label{tbl:transfer dataset}
    \centering
    \begin{tabular}{l c c c c}
        \toprule
        Region & Great London & Great Manchester & West Midlands & South Yorkshire \\
        \midrule
        Average Temperature (°C) & 10.8 & 9.4& 9.7 & 9.2 \\
        Average Precipitation (mm) & 690 & 1047 & 769& 864\\
        Population Density (/km^2) &5,671 & 2,204 & 3,235 & 912\\
        Per Capita GDP (\$) & 75,336 & 38,360 & 33,547 & 28,550 \\
        Average Grid Emissions (t) & 148.99 & 115.27& 110.24 & 45.84 \\
        \bottomrule
    \end{tabular}
\end{table*}

\subsection{A. Datasets}

Since POI data from our three main datasets are not category-aligned due to differences in their collection sources, we did not perform a generalizability test on our main datasets but instead collected data on four distinct ceremonial counties in England for testing. As shown in Table~\ref{tbl:transfer dataset}, the four ceremonial counties vary in their economic level, population scale, and positioning inside England. We further visualize the grid carbon emission distribution of the four counties in Fig.~\ref{fig:transfer}. The figure clearly illustrates significant regional differences in carbon emission distributions.

\begin{figure}[h]
    \vspace{-3mm}
    \centering
    \includegraphics[width=0.9\columnwidth]{figs/emission_distribution.pdf}
    \caption{The grid carbon emission distribution of four England regions: Great London, West Midlands, South Yorkshire, and Warwickshire.}
    \label{fig:transfer}
\end{figure}

\subsection{B. Implementation}
In our implementation, we perform a grid search on all hyperparameters. Specifically, the grid search range for learning rate is set as \{5e-6, 1e-5, 5e-5, 1e-4, 5e-4, 1e-3, 5e-3, 1e-2\}, the range for batch size is \{32, 64, 128\}, the range for the balancing coefficient weight $\alpha$ is \{1e-1, 1e-2, 1e-3\}, and the range for the size of the neighborhood $M$ is set as \{3, 5, 7\}. We set the number of epochs as 500, with an early stopping mechanism to prevent overfitting. Meanwhile, we also fine-tune all hyperparameters of the baselines for fair comparisons. Codes, data, and the fine-tuned hyperparameter values are open-sourced: \url{https://anonymous.4open.science/r/OpenCarbon-2F11}. 

\subsection{C. Preliminary Case Study}
\begin{figure}[h]
    % \centering
\includegraphics[width=0.95\columnwidth]{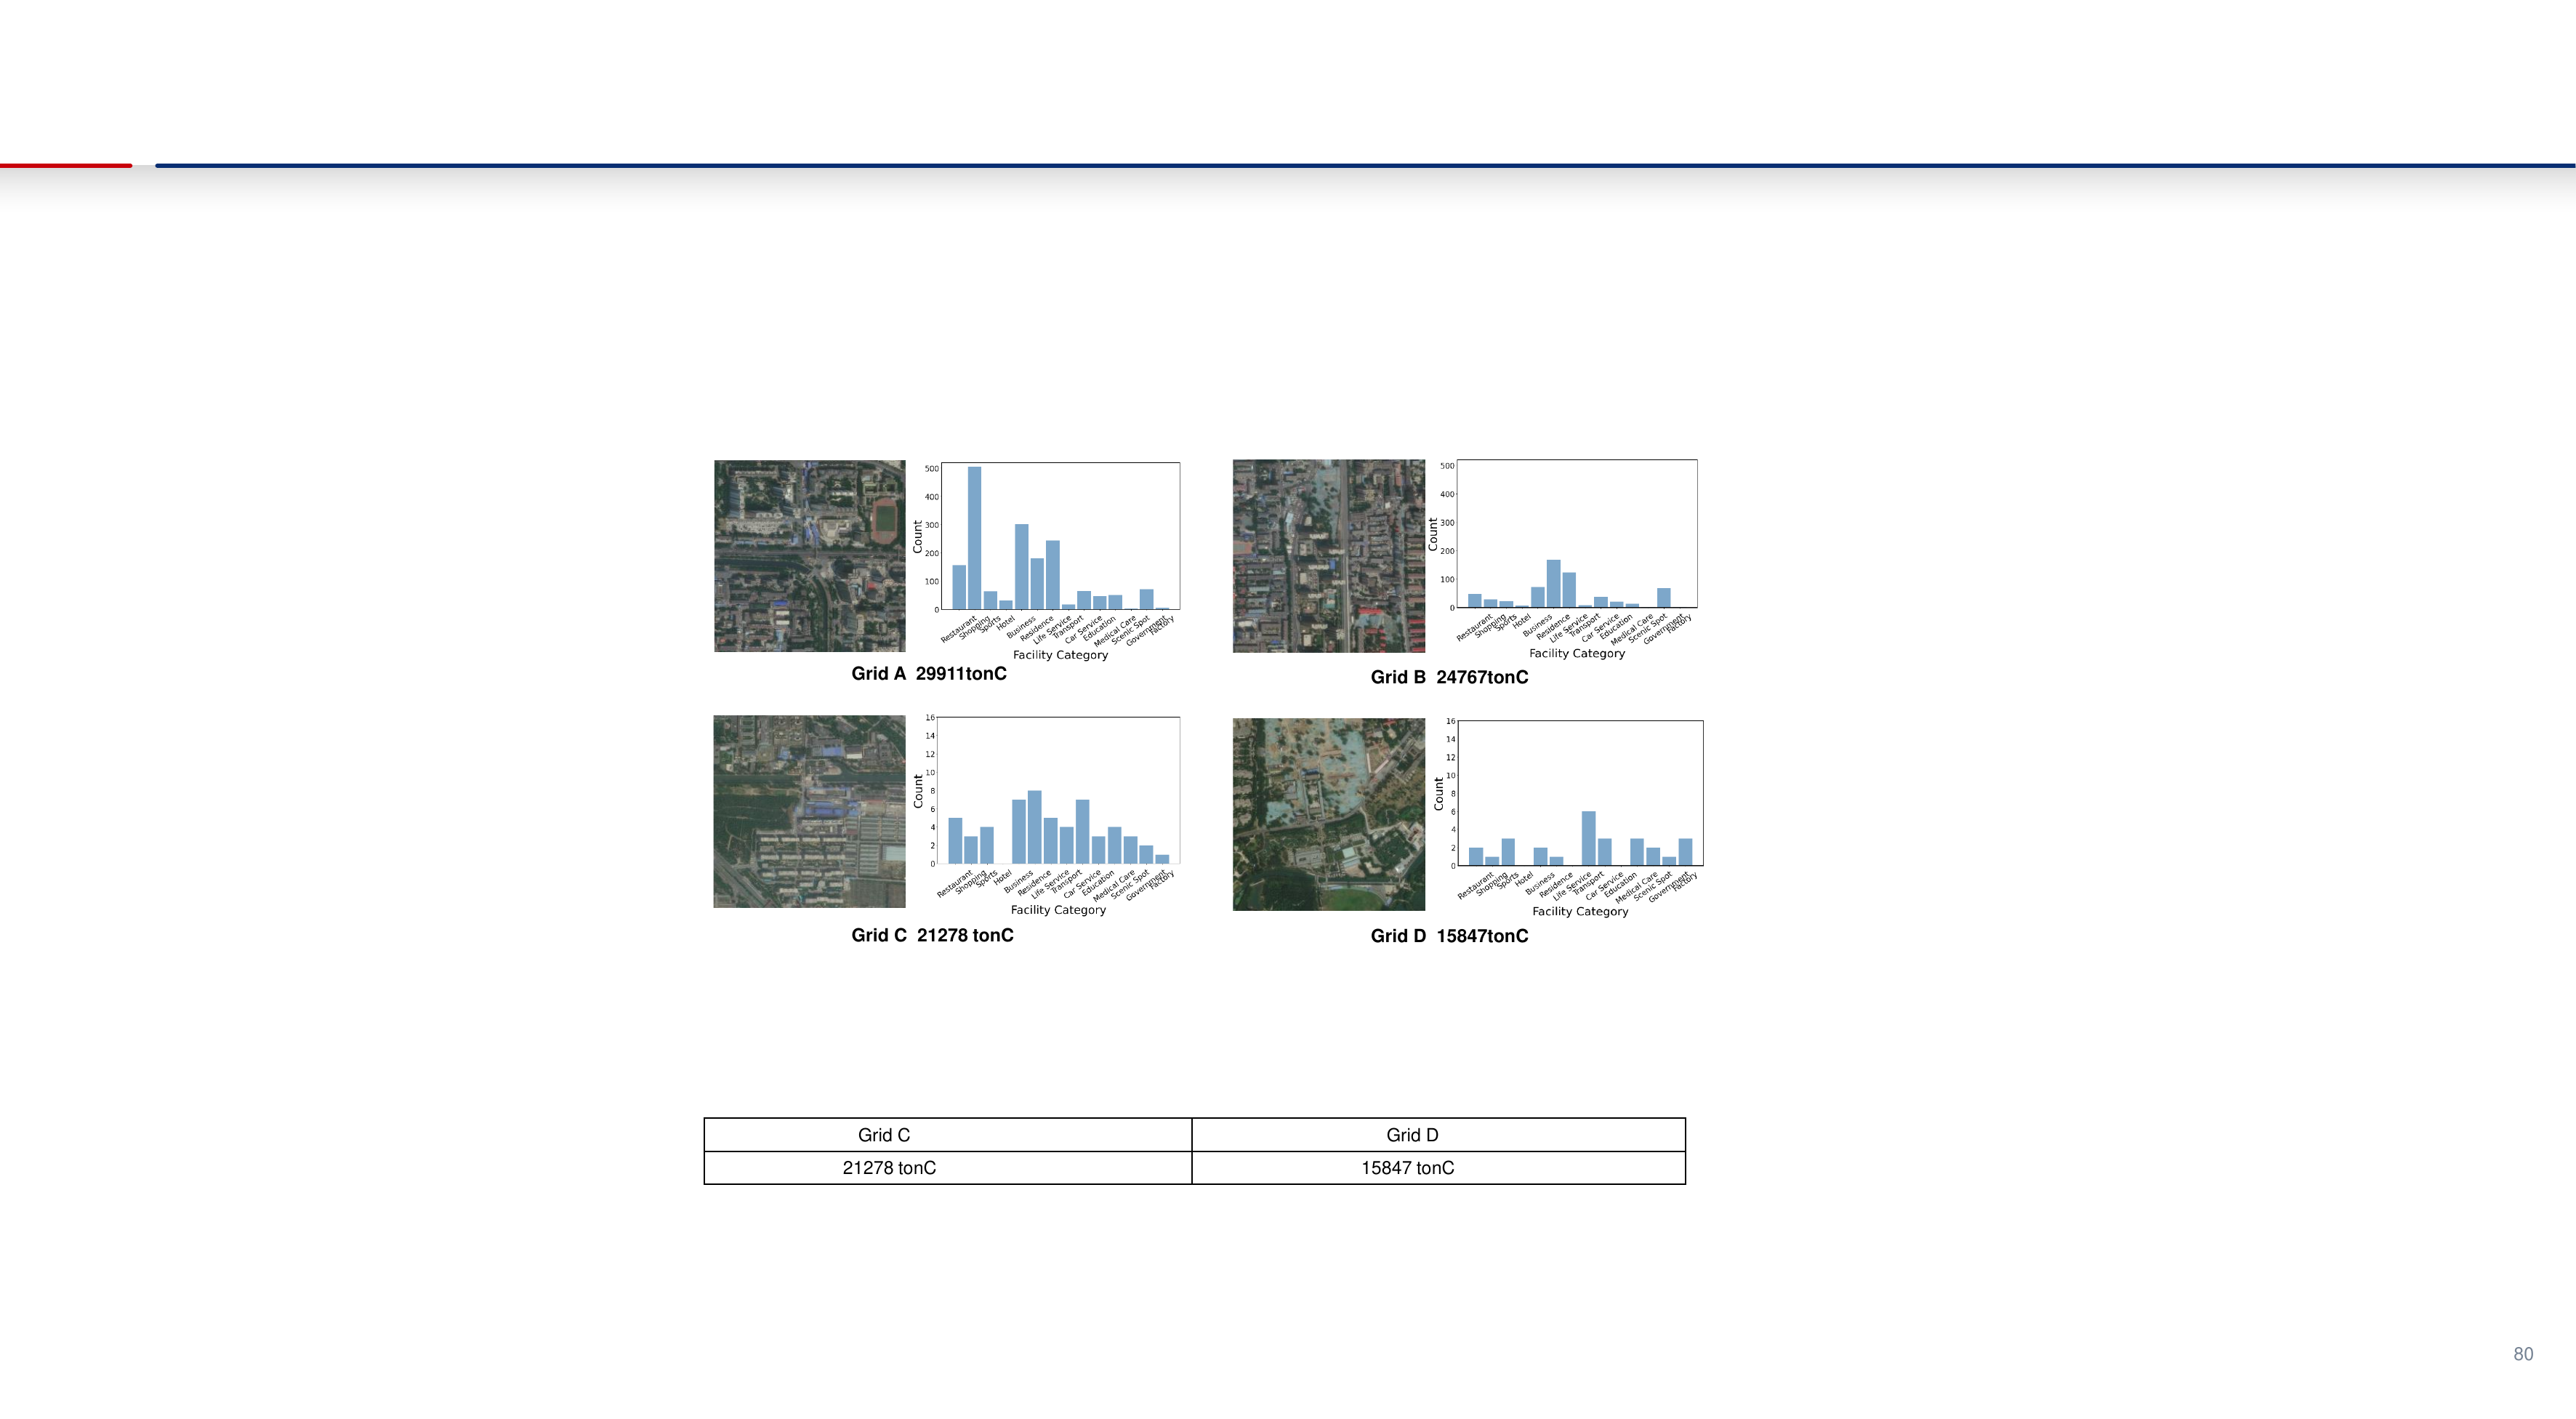}
    \caption{Typical carbon emission cases of 1km $\times$ 1km grids in Beijing. Grid $A$ and $B$ are similar in satellite images yet have different carbon emission levels. Grid $C$ and $D$ have similar facility distribution but are different in carbon emission levels.}
    \label{fig:same_sat}
    \vspace{-4mm}
\end{figure}

% 图要美化
While satellite images provide a relatively macroscopic overview of a city's land layout, POI distribution presents more fine-grained and updated functionality information since it includes the most up-to-date facility information of various function types. Here we present two real cases to show how these two types of data sources complement each other. Grid $A$ and $B$, as shown in Figure~\ref{fig:same_sat}, display similar land use layouts and building densities. making it hard to tell which grid generates higher carbon emissions. However, $A$ has a higher facility density compared with $B$, especially in the shopping category and the business category. Therefore, we can deduce that $A$ has a higher activity intensity which leads to greater carbon emissions. Meanwhile, grids $C$ and $D$ are rural grids with few facilities. But as the satellite images show, $C$ has a larger land use than $D$. Therefore, it is within expectations that $C$ produces higher carbon emissions. These preliminary cases provide evidence for the complementarity of the two data sources and the necessity to leverage both these two sources to predict carbon emissions jointly.
