# Supplementary material for: OpenCarbon: A Contrastive Learning-based Cross-Modality Neural Approach for High-Resolution Carbon Emission Prediction Using Open Data
Source: arXiv:2506.03224 source file (2025-06-03)
Supplement: Supplementary file 3 [file preliminary.tex]

\subsection{Preliminary Case Study}

\subsection{Definitions}
\label{sec:def}
Considering our research goal as high-resolution carbon emission prediction, we introduce a commonly used high-resolution spatial unit in the carbon field, grid: \\  
\noindent
\textbf{Grid:}
In high-resolution carbon emission calculations, the space is usually divided into target square units formed by intersecting horizontal and vertical lines, which are referred to as 'grids'. Common resolutions used for grid division in carbon emission calculations include $1$ km $\times$ $1$ km and $1$ \textdegree $\times$ $1$ \textdegree. 

\noindent
\textbf{Neighborhood:}
The geographically adjacent areas around the target area, typically share common characteristics and functionalities. In this work, we represent the neighborhood of a grid using a grid set of size $M \times M$ centered around the target grid, where $M$ is a hyperparameter.

\begin{figure}[t]
    % \centering
\includegraphics[width=0.95\columnwidth]{figs/cases_new.png}
    \caption{Typical carbon emission cases of 1km $\times$ 1km grids in Beijing. Grid $A$ and $B$ are similar in satellite images yet have different carbon emission levels. Grid $C$ and $D$ have similar facility distribution but are different in carbon emission levels.}
    \label{fig:same_sat}
    \vspace{-4mm}
\end{figure}

% 图要美化
While satellite images clearly show the static land use structure of the city, POI distribution data provides implications for the intensity of different types of activities inside architectures. Here we present two real cases to show how these two types of data sources complement each other. Grid $A$ and $B$, as shown in Figure~\ref{fig:same_sat}, display similar land use layouts and building densities. making it hard to tell which grid generates higher carbon emissions. However, $A$ has a higher facility density compared with $B$, especially in the shopping category and the business category. Therefore, we can deduce that $A$ has a higher activity intensity which leads to greater carbon emissions. Meanwhile, grid $C$ and $D$ are rural grids with few facilities. But as the satellite images show, $C$ has a larger land use than $D$. Therefore, it is within expectations that $C$ produces higher carbon emissions. These preliminary cases provide evidence for the complementarity of the two data sources and the necessity to leverage both these two sources to predict carbon emissions jointly.
